# Supplementary material for: Evaluating the extent to which homeostatic plasticity learns to compute prediction errors in unstructured neuronal networks
Source: arXiv:2202.01521 source file (2022-02-18)
Supplement: Supplementary file 1 [file Supplementary.pdf]

# Supplementary Materials for
# Evaluating the extent to which homeostatic plasticity learns to compute prediction errors in unstructured neuronal networks

Vicky Zhu and Robert Rosenbaum
University of Notre Dame
Notre Dame, IN USA

.

## 1 Adding external input to inhibitory populations does not alter main conclusions.

In the main manuscript, we only considered examples where external input was provided exclusively to excitatory neurons. In this section, we empirically test whether our conclusions were sensitive to the assumption that only excitatory neurons received external input by repeating some simulations from the main text with external input provided to the inhibitory populations as well. Supplementary Figure 1 shows results from a simulation in which top down input was provided to the inhibitory population in addition to population $e_2$ during training. For the mismatched stimulus, the top-down input was removed from the inhibitory population and from population $e_2$. Specifically, in Supplementary Figure 1C,D, we used

$$\left.\begin{aligned} X_{e_1} &= X_e^0 + U \\ X_{e_2} &= X_e^0 + V \\ X_i &= X_i^0 + V \end{aligned}\right\} \text{matched}$$

and

$$\left.\begin{aligned} X_{e_1} &= X_e^0 + U \\ X_{e_2} &= X_e^0 \\ X_i &= X_i^0 \end{aligned}\right\} \text{mismatched}$$

where

$$\begin{aligned} U &= X_e^0/5 \\ V &= -X_e^0/5. \end{aligned}$$

which is identical to Figure 1 from the main text, but with input $V$ provided to $i$ as well. In Supplementary Figure 1E,F, we used

$$\left.\begin{aligned} X_{e_1} &= X_e^0 + c(t)U \\ X_{e_2} &= X_e^0 + c(t)V \\ X_i &= X_i^0 + c(t)V \end{aligned}\right\} \text{matched}$$

and

$$\left.\begin{aligned} X_{e_1} &= X_e^0 + U \\ X_{e_2} &= X_e^0 \\ X_i &= X_i^0 \end{aligned}\right\} \text{mismatched.}$$

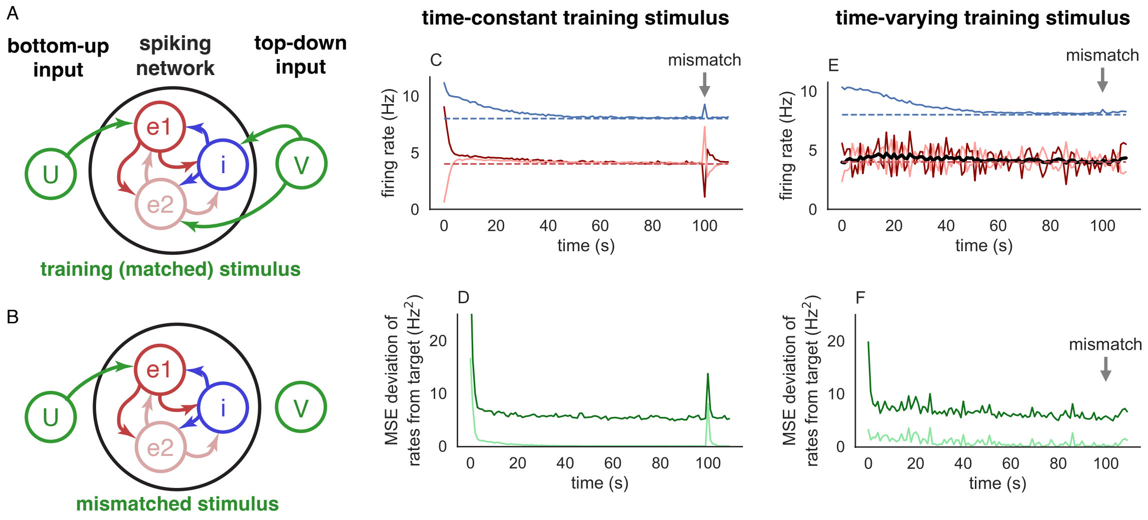


Supplementary Figure. 1: **Similar results are obtained with input to inhibitory populations. A,B)** Network schematics. Same as Figure 1A,B except top-down external input was provided to the inhibitory population as well. **C,D)** Same as Figure 1C,D except top-down external input was provided to the inhibitory population as well. **E,F)** Same as Figure 5C,D except top-down external input was provided to the inhibitory population as well.

where

$$U = X_e^0/20$$
$$V = -X_e^0/20.$$

This is identical to Figure 5 from the main text, but with input $V$ provided to $i$ as well. Our results (Supplementary Figure 1) show a strong mismatch response after training on time-constant input, but not time-varying input.

We additionally tested whether similar results were obtained for distributed external input provided to the inhibitory and excitatory populations (Supplementary Figure 2). Specifically, in Supplementary Figure 2C,D, we used

$$\left.\begin{aligned} X_e &= X_e^0 + \vec{U}_e + \vec{V}_e \\ X_i &= X_i^0 + \vec{U}_i + \vec{V}_i \end{aligned}\right\} \text{ matched}$$

and

$$\left.\begin{aligned} X_e &= X_e^0 + \vec{U}_e \\ X_i &= X_i^0 + \vec{U}_i \end{aligned}\right\} \text{ mismatched.}$$

where $\vec{U}_a$ and $\vec{V}_a$ are normally distributed $N_a$-dimensional vectors,

$$\vec{U}_a \sim \sigma_s N(0,1)$$
$$\vec{V}_a \sim \sigma_s N(0,1)$$

for $a = e, i$. This is identical to Figure 4 from the main text except distributed input was provided to

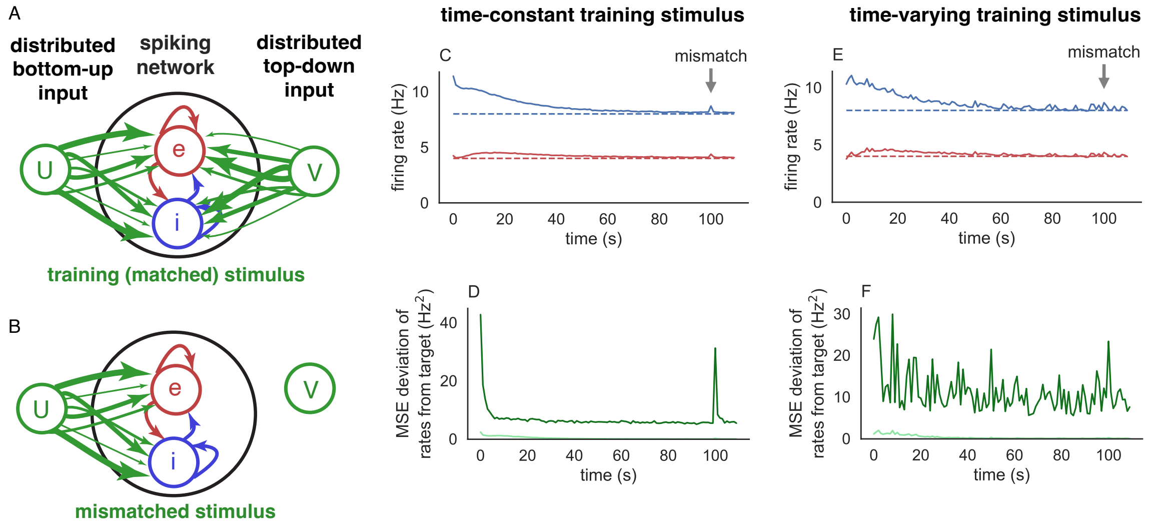


Supplementary Figure. 2: **Similar results are obtained with distributed inputs to inhibitory populations. A,B)** Network schematics. Same as Figure 4A,B except distributed external input was provided to the inhibitory population as well. **C,D)** Same as Figure 4C,D except top-down external input was provided to the inhibitory population as well. **E,F)** Same as Figure 9C,D except top-down external input was provided to the inhibitory population as well.

the inhibitory population as well. In Supplementary Figure 2E,F, we used

$$\left.\begin{aligned} X_e &= X_e^0 + c(t)\vec{U}_e + c(t)\vec{V}_e \\ X_i &= X_i^0 + c(t)\vec{U}_i + c(t)\vec{V}_i \end{aligned}\right\} \text{ matched}$$

and

$$\left.\begin{aligned} X_e &= X_e^0 + \vec{U}_e \\ X_i &= X_i^0 + \vec{U}_i \end{aligned}\right\} \text{ mismatched.}$$

which is identical to Figure 9 from the main text except distributed input was provided to the inhibitory population as well. Our results (Supplementary Figure 2) show a strong mismatch response after training on time-constant distributed input, but not time-varying distributed input.

In conclusion, adding external input to the inhibitory population does not qualitatively affect our overall findings.

## 2 Increasing the strength of mismatched stimuli produces pronounced mismatch responses.

We next repeated the simulation from Figure 5 of the main manuscript, but increased the strength of the mismatched stimulus. In particular, we set

$$\left.\begin{aligned} X_{e_1} &= X_e^0 + c(t)U \\ X_{e_2} &= X_e^0 + c(t)V \\ X_i &= X_i^0 \end{aligned}\right\} \text{ matched}$$

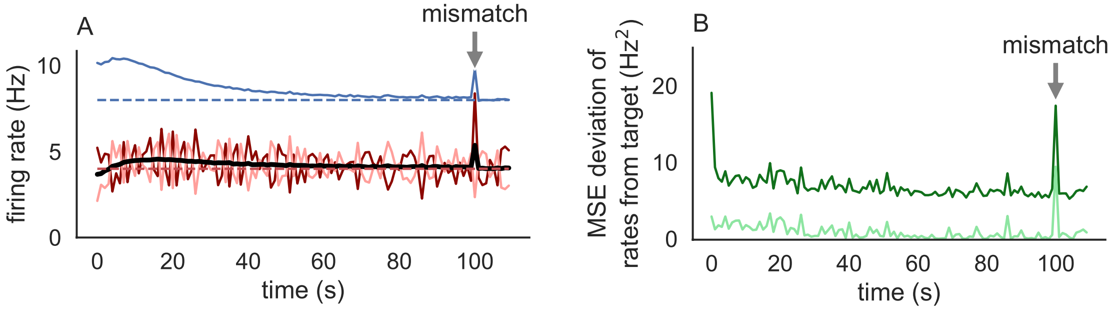


Supplementary Figure. 3: **Mismatch responses are observed with stronger mismatched stimuli. A,B)** Same as Figure 5 except the strength of the mismatched input was increased by six-fold.

and

$$\left.\begin{aligned} X_{e_1} &= X_e^0 + 6U \\ X_{e_2} &= X_e^0 \\ X_i &= X_i^0 \end{aligned}\right\} \text{mismatched.}$$

In this case, the mismatched stimulus has a larger magnitude than any of the matched stimuli used for training (in addition to the mismatch that occurs). As predicted, we observed a pronounced mismatch response in this case (Supplementary Figure 3)

## 3 Including several excitatory and inhibitory populations does not change our conclusions.

In all examples considered so far, we considered a single inhibitory population and one or two excitatory populations. We next tested whether including more populations would affect our results. Specifically, we repeated the simulations from Figure 5, but we broke the excitatory and inhibitory populations each into three subpopulations (Supplementary Figure 4). During training (matched stimuli), populations $e_1$ and $i_1$ received bottom-up input from $U$, populations $e_2$ and $i_2$ received top-down input from $V$. And populations $e_3$ and $i_3$ received no external input. Specifically,

$$\left.\begin{aligned} X_{e_1} &= X_e^0 + c(t)U \\ X_{e_2} &= X_e^0 + c(t)V \\ X_{e_3} &= X_e^0 \\ X_{i_1} &= X_i^0 + c(t)U \\ X_{i_2} &= X_i^0 + c(t)V \\ X_{1_3} &= X_i^0 \end{aligned}\right\} \text{matched}$$

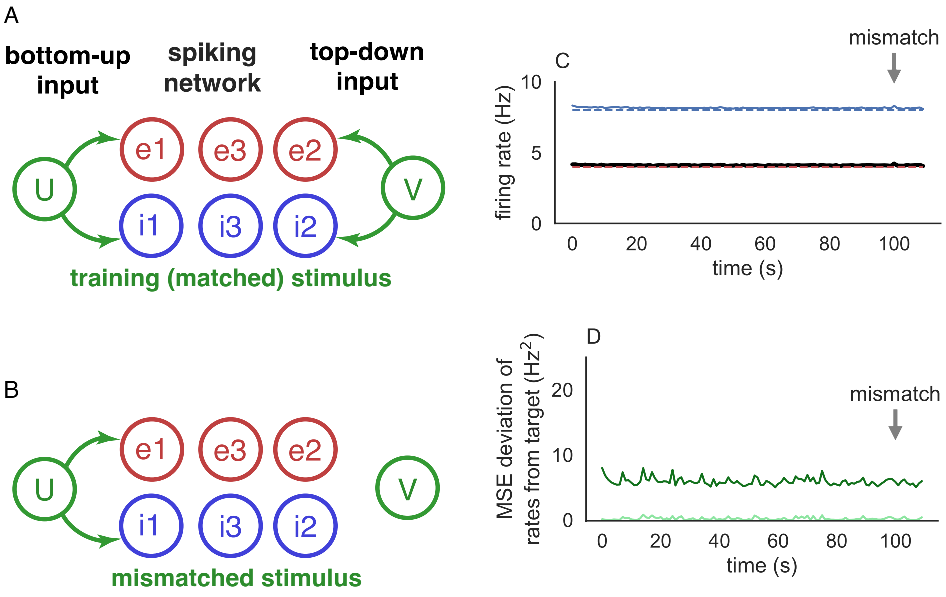


Supplementary Figure. 4: **Mismatch responses are not observed when more populations are considered.** Same as Figure 5 except more populations were added. Connections between populations are not shown for simplicity of the diagram.

and

$$\left.\begin{aligned} X_{e_1} &= X_e^0 + U \\ X_{e_2} &= X_e^0 \\ X_{e_3} &= X_e^0 \\ X_{i_1} &= X_i^0 + U \\ X_{i_2} &= X_i^0 \\ X_{1_3} &= X_i^0. \end{aligned}\right\} \text{mismatched.}$$

Our results (Supplementary Figure 4C,D) shows no visible mismatch response, consistent with our original findings from Figure 5. Hence, simply adding more populations does not change our overall findings. This is consistent with the conclusions reached by our theoretical arguments in the main text.
